# Supplementary material for: Video-DPRP: A Differentially Private Approach for Visual Privacy-Preserving Video Human Activity Recognition
Source: arXiv:2503.02132 source file (2025-03-03)
Supplement: Supplementary file 1 [file X_suppl.tex]

\clearpage
\setcounter{page}{1}
\maketitlesupplementary
\begin{figure}[t!]
\includegraphics[width=1\linewidth]{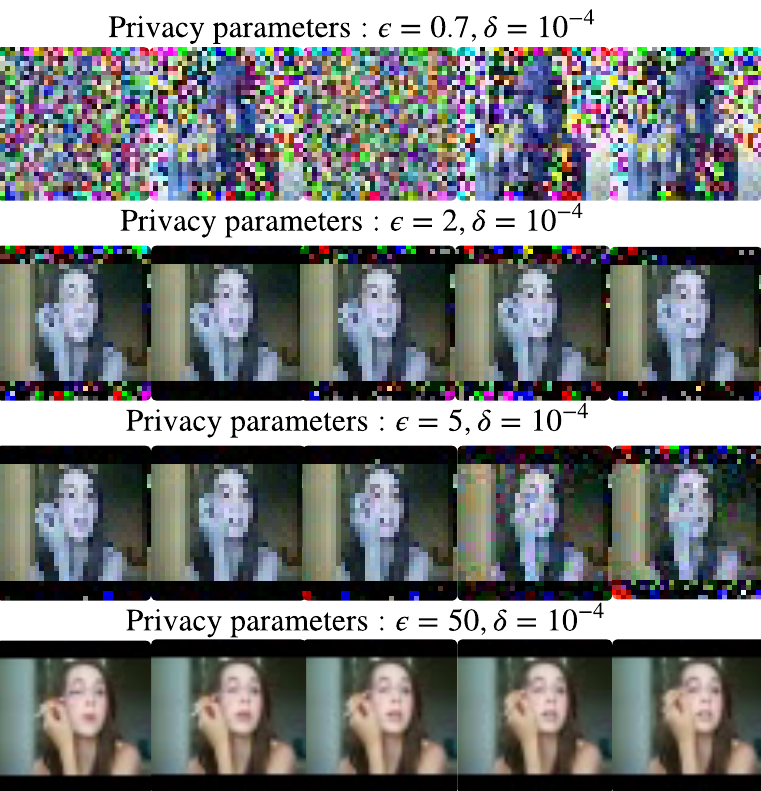}
    \caption{\textbf{Qualitative analysis of Video-DPRP}. From top to bottom, the rows represent reconstructed videos using differential privacy parameters $\epsilon \in \{0.7,2,5,50\}$, $\delta=10^{-4}$ and $k= 32\times 32 \times 3$.} \label{video_dprp_v}
\end{figure}
\begin{figure*}[t!]
\includegraphics[width=1\linewidth]{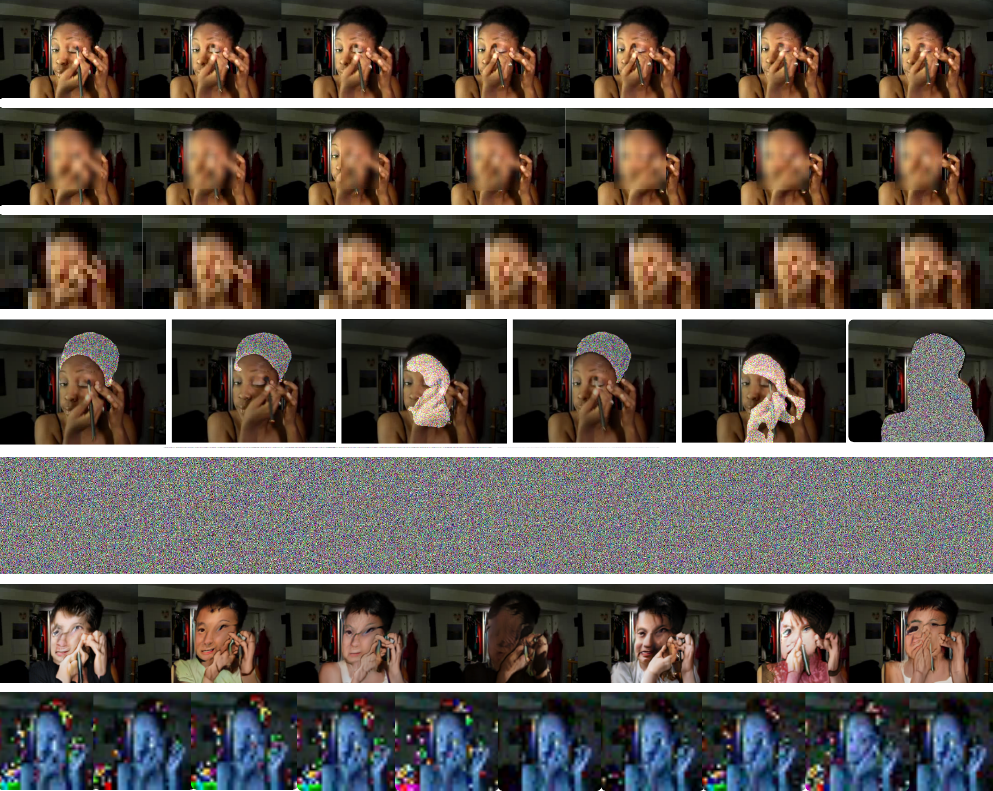}
    \caption{\textbf{Qualitative analysis of privacy-preserving techniques}. The video represents a sample from the \textbf{Apply Makeup} class of the UCF101\cite{soomro2012ucf101} dataset. From top to bottom, the rows represent: (1) Original video, (2) Face-blurred video \cite{jaichuen2023blur}, (3) Inverse-super resolution \cite{ryoo2017privacy}, (4) Selective privacy \cite{ilic2024selective}, (5) Appearance-free \cite{ilic2022appearance}, (6) Full body anonymization \cite{hukkelaas2023realistic}, and (7) Video-DPRP (\textbf{ours}).} \label{videos}
\end{figure*}
In this supplementary material, we provide additional details on: (i) the implementation of some state-of-the-art privacy-preserving techniques described in Section \ref{details}, (ii) the proof of privacy guarantees for Algorithm \ref{alg:example} (Section \ref{sec:rationale}), and (iii) some qualitative analyses of Video-DPRP and its robustness to adversary attacks (Section \ref{robust}).
\section{Implementation details}
%\textbf{Video-DPRP on Images}\\
%Although Video-DPRP was originally developed for differentially private video reconstruction, it can also be adapted for application on images.\\
\textbf{Obfuscation Methods}\\
\underline{Selective privacy} \cite{ilic2024selective} is a stand alone framework designed to obfuscate privacy-sensitive regions within a video, without compromising on action recognition performance. The framework consists of: (i) a template library, $\tau$, containing various privacy attributes, (ii) a matcher that generates saliency maps between selected privacy attributes and frames where privacy needs to be preserved, and (iii) an obfuscator that uses the generated saliency maps to conceal privacy attributes in a temporally consistent manner. Obfuscation is achieved through optical flow, similar to the approach proposed by Ilic \etal \cite{ilic2022appearance}. In our experiments, we used the privacy attributes $\tau = \{\textit{"forehead", "hair", "left-eye", "right-eye","skin"}\}$.\\
\underline{Face Blurring} \cite{jaichuen2023blur}: For face blurring, other YOLO algorithms or face detection techniques could have been used. Here, we chose YOLOv3 \cite{redmon2016you} solely for its effectiveness in detecting faces, which are then used for further pre-processing (blurring of the bounding boxes).\\
\textbf{Anonymization methods}\\
\underline{DeepPrivacy2} \cite{hukkelaas2023deepprivacy2} is a generative adversarial image anonymization framework that first detects human figures and then uses an inpainting adversarial network for unconditional image generation. To asses its performance on video activity recognition, we anonymized each video on a frame-by-frame basis before using it for activity recognition. We used the \href{https://www.hukkelas.no/deep_privacy2/#/README}{\texttt{code}} provided by the authors along with their instructions for the anonymization process.
\begin{figure*}[t!]
\includegraphics[width=1\linewidth]{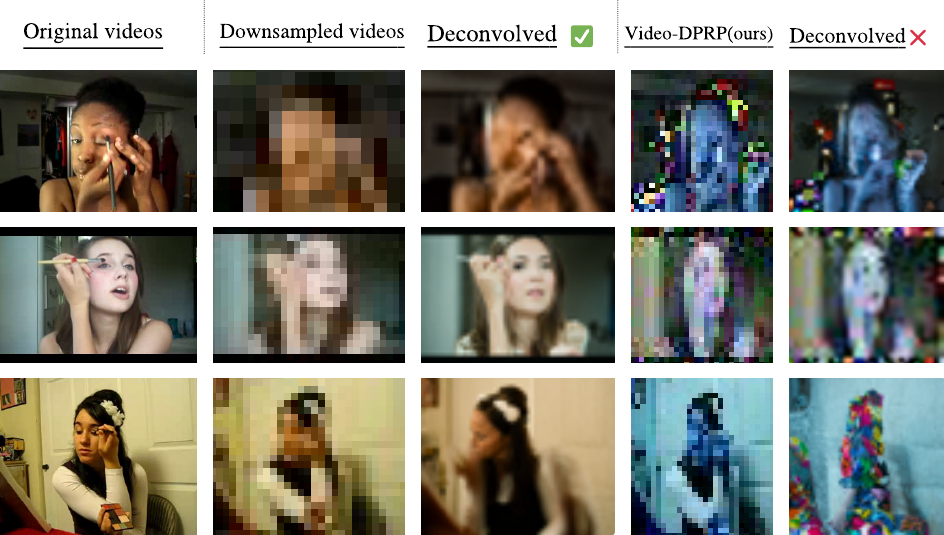}
    \caption{\textbf{Robustness to deconvolution}. We use SUPIR \cite{yu2024scaling} to recover privacy attributes from privacy preserved videos. Specifically, we apply it to downsampled videos (using ISR \cite{ryoo2017privacy} resolution $16 \times 12$) and Video-DPRP (using privacy parameters $\epsilon=2, \delta=10^{-4}$).} \label{deconv_videos}
\end{figure*}
\section{Privacy Guarantee of Video-DPRP}\label{sec:rationale}
We rely on the rigorous proof of differentially private random projections from Tu \etal \cite{tudifferentially}, as also referenced in the work of Kenthapadi \etal \cite{kenthapadi2012privacy} for small dataset release using random projections. The proof is reported here for completeness, with the notation kept consistent with those used in our main paper.
Let $\left|\right|\cdot\left|\right|$, $\left|\right|\cdot\left|\right|_{F}$ and $\left<\cdot,\cdot \right>$ denotes the $L_{2}$ norm, the Frobenius norm and the Euclidean inner product respectively. Let $\mathcal{R}$ be a $d \times k$ randomized Gaussian projection matrix, where each entry is drawn independently from $\mathcal{N}(0, \sigma_{p}^{2})$, with $\sigma_{p}=1/\sqrt{k}$. Let $X$ and $X'$ be two $T \times d$ video matrices as described in Section \ref{overview}, that differ only in one row $i$ with $\left|\right|X_{i}-X_{i}'\left|\right| \leq \theta$. The privacy guarantee of Video-DPRP relies on the proof that both the random projection and the covariance matrix in Algorithm \ref{alg:example} are differentially private.\\
\begin{table}
    \centering
    \begin{tabular}{lcc}
      \toprule
      \multirow{4}{*}{}
      &\multicolumn{2}{c}{Reconstruction (sec/Video)}\\
      \midrule
      \underline{$\textbf{Methods}$} & \textbf{UCF101} &\textbf{HMBD51} \\
      
      V-SAM\cite{hukkelaas2023deepprivacy2} & 33.12 & 35.07 \\
      
      ISR$_{(32\times 24)}$\cite{ryoo2017privacy}&\textbf{19.24} & \textbf{18.97}\\
      Deepprivacy \cite{hukkelaas2023realistic} & 35.60& 38.93 \\
      Face Anonymizer \cite{ren2018learning} & 30.21& 26.74 \\
      Appearance free \cite{ilic2022appearance} & 23.74& 21.60 \\
      Selective privacy \cite{ilic2024selective} & 29.81& 27.18 \\
      Face blurring \cite{jaichuen2023blur} & 26.08 & 24.49 \\
      Video-DPRP(ours) & \underline{20.32} & \underline{19.84} \\
      \bottomrule
    \end{tabular}
    \caption{Reconstruction time per video (in seconds) for \textbf{UCF101} \cite{soomro2012ucf101} and \textbf{HMDB51} \cite{kuehne2011hmdb}. The best (lowest) time is highlighted in \textbf{bold}, and the second best is \underline{underlined}.}\label{reconstrict}
\end{table}
\begin{figure}[t]
\includegraphics[width=1\linewidth]{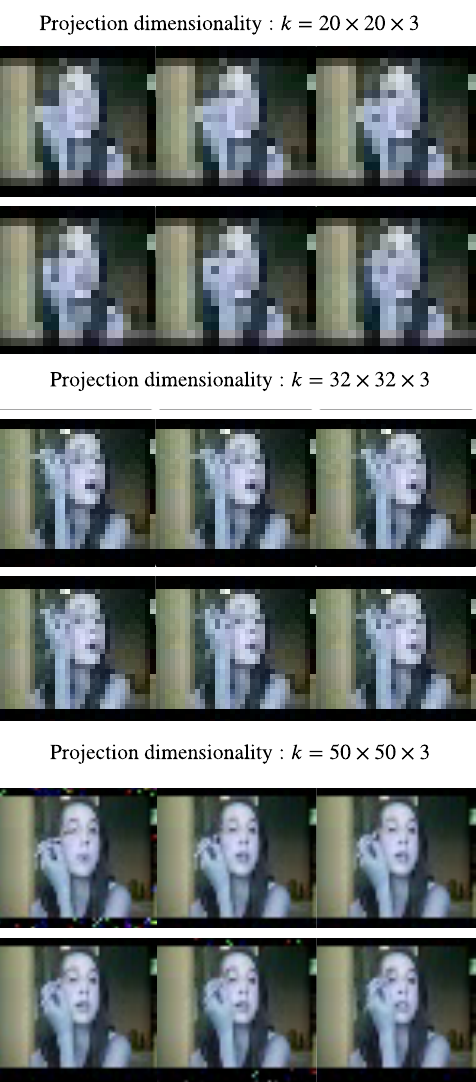}
    \caption{\textbf{Qualitative analysis of Video-DPRP}. For constant values of $b = 0.8$, $\epsilon = 5$, and $\delta = 10^{-4}$, increasing the dimensionality value $k$ results in better-quality videos. A larger $k$ effectively retains more of the original dimensionality, enabling the random projection to capture more of the variance or structure of the original video, thereby minimizing information loss.
    At very small values of $k$, significant compression occurs, resulting in greater information loss and higher distortion. This explains why higher $k$ values improve activity recognition performance but compromise visual privacy preservation. } \label{video_dprp_k}
\end{figure}
\textbf{\underline{Proof of Theorem \ref{theo3}}}\\
To begin, we need to prove a Lemma.
\begin{lemma}\label{lem5}
With probability of at least $1-\delta_{1}$ we have
    \[
    \left|\right|X\mathcal{R}-X'\mathcal{R}\left|\right|_{F} \leq \theta\sigma_p\sqrt{k+2\sqrt{klog({1}/{\delta_1})}+2log({1}/{\delta_1})}
    \] 
\end{lemma}
\begin{proof}
    Since $X$ and $X'$ only differ in one row $i$, we have $(X\mathcal{R}-X'\mathcal{R})_{mn}=0$ for $m \neq i$ and that 
    \[(X\mathcal{R}-X'\mathcal{R})_{ij}= \left<X_i,\mathcal{R}_j \right>-\left<X'_i,\mathcal{R}_j \right>=\left<X_i-X_i',\mathcal{R}_j\right>
    \]
    Where $\mathcal{R}_j$ is the $j$-th colomn of $\mathcal{R}$. Let $\theta=X_i-X_i'$. By scaling properties of Gaussians (example if $a$ and $b$ are constants, $X \sim \mathcal{N}(0,\sigma^2_{x})$ and $Y \sim \mathcal{N}(0,\sigma^2_{y})$, then $aX+bY  \sim \mathcal{N}(0,a^2\sigma^2_{x}+b^2\sigma^2_{y})$), we know $\left<\theta,\mathcal{R}_j\right> \sim \mathcal{N}(0,\left|\right|\theta\left|\right|^2\sigma^2_p)$. Let $Y_j \sim \mathcal{N}(0,1)$ and $\mathcal{X}^2_{k}$ denotes a random variable drawn from a Chi-square distribution with $k$ degrees of freedom. We now bound the matrix norm as follows
    \[
    \left|\right|X\mathcal{R}-X'\mathcal{R}\left|\right|_{F}=\sqrt{\sum_{j=1}^{k}\left<\theta,\mathcal{R}_j\right>^2}= \sqrt{\sum_{j=1}^{k}(\left|\right|\theta\left|\right|\sigma_pY_{j})^2}
    \]
    \[
    = \left|\right|\theta\left|\right|\sigma_p\sqrt{\mathcal{X}^2_{k}}
    \]
    The second equality follows since if $X \sim \mathcal{N}(0,\sigma^2)$, then $X/\sigma \sim \mathcal{N}(0,1)$. From Laurent \etal \cite{laurent2000adaptive}, we have the following tail bound on a random variable $X$ drawn from a Chi-squared distribution with $k$ degree of freedom
    \[
    Pr[X\geq k+2\sqrt{kx}+2x] \leq \exp{(-x)}
    \]
    By setting $x=log({1}/{\delta})$, we complete the proof.
\end{proof}
\begin{lemma}
    The mechanism $M(D)=f(D)+G$, where $G$ is a random Gaussian matrix with entries drawn from $\mathcal{N}(0,\sigma^2_1)$, satisfies $(\epsilon,\delta)$-differentially privacy, if $\delta<\frac{1}{2}$, where $\sigma^2_1=2\Delta(f)^2(log(1/2\delta)+\epsilon)/\epsilon^2$ and $\Delta(f)$ is the sensitivity
\end{lemma}\label{lem3}
With the support of Lemma 5 and Lemma 6, we are now ready to prove Theorem \ref{theo3} from the main paper.
\begin{proof}
    By replacing $\Delta(f)$ in Lemma 6 with the right-hand side from Lemma 5, and using $\delta_1/2$, we obtain 
    \footnotesize\[
        \sigma_1= \theta\sigma_p\sqrt{k+2\sqrt{klog({2}/{\delta_1})}+2log({2}/{\delta_1})}{\sqrt{2(log(1/2\delta_1)+\epsilon_1)}}/{\epsilon_1}
    \]
\end{proof}
\hspace{-0.05\linewidth}\textbf{\underline{Proof of Theorem \ref{theo4}}}
\begin{proof}
    The privacy guarantee defined in Theorem \ref{theo4} follows directly from \cite{dwork2014analyze} and is also reported in \cite{gondara2020differentially}. 
\end{proof}

\subsection{The $L_{2}$ sensitivity bound $\theta$}
In Section \ref{guarantee}, we set $\theta={255}/{\sqrt{k}}$. We provide additional details for this setting below.\\   
\textbf{\underline{Frobenius Norm of $X$}}\\
The Frobenius norm of the video matrix $X \in \mathbb{R}^{T\times d}$ is defined as:
\[\footnotesize \left|\right|X\left|\right|_{F}= \sqrt{\sum_{i=1}^T\sum_{j=1}^d\left|X_{ij}\right|^{2}}\] 

where $X_{ij}$ denotes the element in the $i$-th row and $j$-th column of the video $X$.\\
\textbf{\underline{$L_{2}$ Sensitivity of $\left|\right|X\left|\right|_{F}$}}\\
To compute the $L_{2}$ sensitivity of the Frobenius norm, we consider the video matrices $X$ and $X'$ that differ by exactly one entry. Let $X'$ be obtained from $X$ by modifying a single pixel, say at position $(i,j)$. The Frobenius norm difference between $X$ and $X'$ is :
\[\footnotesize \left|\right|X\left|\right|_{F}-\left|\right|X'\left|\right|_{F}=\left|\sqrt{\sum_{i=1}^T\sum_{j=1}^d\left|X_{ij}\right|^{2}}-\sqrt{\sum_{i=1}^T\sum_{j=1}^d\left|X'_{ij}\right|^{2}}\right|\]
Because $X$ and $X'$ differ by exactly one entry, this simplifies to:
\[\footnotesize \left|\right|X-X'\left|\right|_{F}=\sqrt{(X_{ij}-X_{ij})^{2}}\]
The $L_{2}$ sensitivity of the Frobenius norm function, $\Delta$, is the maximum possible change in the Frobenius norm due to a single change in one entry of the video matrix:
\[\footnotesize \Delta=\underset{X,X'}{sup}\left|\right|X-X'\left|\right|_{F}\]
Where \textit{sup} denotes the supremum. Since $X$ and $X'$ differ by only one entry:
\[\footnotesize \footnotesize \Delta=\underset{X_{ij},X_{ij}'}{sup}\sqrt{(X_{ij}-X'_{ij})^{2}}=\underset{X_{ij},X_{ij}'}{sup}{\left|X_{ij}-X'_{ij}\right|}\]
Since each entry of $X_{ij}$ and $X_{ij}'$ are bounded within the range $[0,255]$ then:
\[\footnotesize \Delta=\left|255-0\right|\]
Given the function $f(X)=X\mathcal{R}$ in Theorem \ref{theo3}, the sensitivity is given by:
\[\footnotesize \theta=\underset{X,X'}{sup}\left|\right|X\mathcal{R}-X'\mathcal{R}\left|\right|_{F}=\underset{X,X'}{sup}\left|\right|(X-X')\mathcal{R}\left|\right|_{F}.\]
Since $X$ and $X'$ differ by only one entry at position $(i,j)$ then the Frobenius norm reduces to the $L_{2}$ norm of the product of the difference between $(X_{ij}-X_{ij}')$ and the corresponding row of $\mathcal{R}$:
\[\footnotesize \left|\right|(X-X')\mathcal{R}\left|\right|_{F}=\left|\right|(X_{ij}-X_{ij}')\mathcal{R}_{j}\left|\right|_{2},\]
Where $\mathcal{R}_j$ denotes the $j$-th row of the matrix $\mathcal{R}$. Since $\mathcal{R}$ has entries drawn from $\mathcal{N}(0,\sigma_p)$, the $L_{2}$ norm of the row $R_{j}$ satisfies:
\[\footnotesize \left|\right|R_{j}\left|\right|_{2} \approx \frac{1}{\sqrt{k}}\]
Thus, the Frobenius norm becomes:
\[\footnotesize \left|\right|(X_{ij}-X_{ij}')\mathcal{R}_{j}\left|\right|_{2}=\left|X_{ij}-X_{ij}'\right|\frac{1}{\sqrt{k}}\]
Since $X_{ij}$ and $X'_{ij}$ are bounded by $[0,255]$, their maximum possible difference is:
\[\footnotesize \left|X_{ij}-X'_{ij}\right|\leq 255\]
We conclude that, when $X$ and $X'$ differ by exactly one entry, the $L_{2}$ sensitivity of $f(X)=X\mathcal{R}$ is :
\[\footnotesize \theta=\underset{X,X'}{sup}\left|\right|(X-X')\mathcal{R}\left|\right|_{F}=\frac{255}{\sqrt{k}}.\]
\section{Robustness to Deconvolution}\label{robust}
We consider a scenario where an attacker launches an adversarial attack and successfully gains access to the privacy-preserved videos. One potential method for recovering the video's privacy attributes is through deconvolution. To test the robustness of Video-DPRP to deconvolution, we used a SOTA image restoration technique SUPIR, proposed by Yu \etal \cite{yu2024scaling} to recover the original videos. SUPIR leverages advanced generative priors, model scaling with over 20 million high-resolution annotated images, and innovative architectural designs such as the ZeroSFT connector for precise pixel-level control. The model incorporates textual prompts to enable controllable image restoration and introduces restoration-guided sampling to ensure fidelity to the input image. SUPIR significantly enhances the restoration of severely degraded images and offers flexible, targeted adjustments, showcasing SOTA performance in both synthetic and real-world benchmarks. We apply the pre-trained SUPIR model (available on this \href{https://supir.xpixel.group}{\texttt{website}}) to Video-DPRP with privacy parameters $\epsilon=2, \delta=10^{-4}$ and to downsampled videos  with resolution $16 \times 12$ (ISR \cite{ryoo2017privacy}).

As illustrated in Figure \ref{deconv_videos}, SUPIR is able to recover a significant amount of privacy attributes from ISR \cite{ryoo2017privacy}, such as gender and skin color. In contrast, recovering such attributes from Video-DPRP proves to be significantly more challenging.\\
\begin{figure}[t!]
\includegraphics[width=0.9\linewidth]{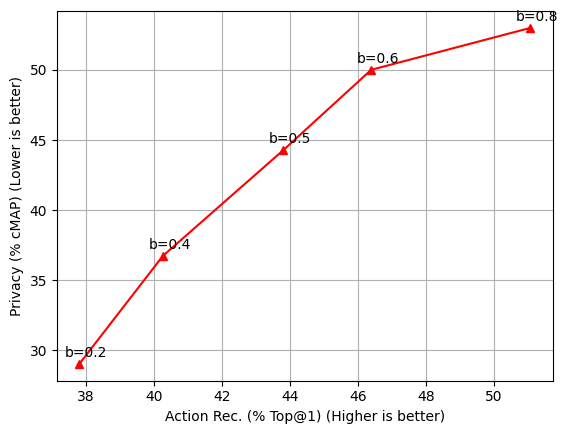}
    \caption{\textbf{Graphical result}. Following Table \ref{budget}, varying the parameter $b$ while keeping $\delta = 10^{-4}$ and $k = 32 \times 32 \times 3$ shows improved action recognition performance but a significant decrease in privacy performance. Conducting a grid search on $b$ may help identify an optimal value that balances both utility and privacy effectively.} \label{graph}
\end{figure}
\begin{figure}[t!]
\includegraphics[width=0.9\linewidth]{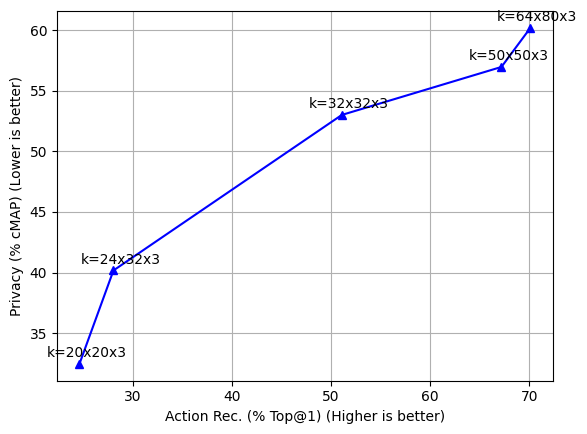}
    \caption{\textbf{Graphical result}. Following Table \ref{dimensionality}, varying the parameter $k$ while keeping $\delta = 10^{-4}$ and $b =0.8$ shows improved action recognition performance but a significant decrease in privacy performance. Conducting a grid search on $k$ may help identify an optimal value that balances both utility and privacy effectively.} \label{graph2}
\end{figure}
\section{Computational efficiency}
We measured the time taken to reconstruct privacy-preserved videos from the UCF101 and HMDB51 datasets using different methods, as shown in Table \ref{reconstrict}. Although Video-DPRP has a polynomial time complexity as outlined in Section \ref{overview}, it remains computationally efficient with an average reconstruction rate of $\sim$ \textbf{20 sec/Video} for both datasets. In contrast methods such as Selective Privacy\cite{ilic2024selective}, Face Anonymizer \cite{ren2018learning}, V-SAM\cite{hukkelaas2023realistic}, Appearance-Free\cite{ilic2022appearance}, and Face Blurring\cite{jaichuen2023blur} incur additional computational overhead due to their use of external models such as  surface-guided GANs, YOLO, and optical flow.
